# Supplementary material for: Probing molecular-motor forces driving Chlamydomonas gliding motility by holographic microscopy
Source: arXiv:2512.13209 source file (2026-09-29)
Supplement: Supplementary file 1 [file fares2025_SI.pdf]

# Inferring intraciliary dynamics from the gliding motility of *Chlamydomonas reinhardtii*
# – Supplementary Information –

Nicolas Fares,[1,*] Elorri Garcia,[1,†] Ahmad Badr,[1] Yacine Amarouchene,[1] Alexandros A. Fragkopoulos,[2,‡] Oliver Bäumchen,[2] Thomas Salez,[1,§] and Antoine Allard[1,¶]

[1] *Univ. Bordeaux, CNRS, LOMA, UMR 5798, F-33400, Talence, France.*
[2] *Experimental Physics V, University of Bayreuth, Bayreuth, Germany.*
(Dated: December 12, 2025)

## I. COMPARATIVE EXPERIMENTS: EXPERIMENTS ON GROUPS OF CELLS

Comparative experiments were performed on groups of gliding cells, following the work done in Ref. [28] of the main document. Protocols and experimental techniques are described hereafter. Let us point out that, here, those experiments serve as calibrations and verifications of the experiments described in the main document, which are performed on single cells *via* Mie holography. Note that the experiments on groups of cells are referred to as "comparative experiments (on groups of cells)" in the next sections.

### Cultivation of the cells

Extensive details can be found in Refs. [28,38] of the main document. Suspensions of cells are grown in a commercial tri-acetate-phosphate (TAP) growth medium purchased (Gibco TAP Growth Media, optimized for Chlamydomonas culture). After three days of growth in the culture medium (*i.e.* three days of exponential growth) inside an incubator, a suspension is centrifuged for 10 minutes at an acceleration of $100g$ ($g$ denoting the gravity constant). Then, the cells are re-suspended in fresh TAP medium (600 $\mu$L) to optimize nutrient availability and let in the incubator for roughly one hour for the cells to grow back their flagella. The concentration of the suspension is determined by counting cells in a Neubauer chamber and diluted to the desired concentration. Finally, the suspension is put in a chamber that consists of two glass coverslips separated by a 1-millimeter-thick layer of polydimethilsiloxane (PDMS, Sylgard 184 from Dow Corning). Actually, the PDMS layer is a two-step layer, allowing for the presence of layer of air on top of the suspension. This layer of air prevents cells from sticking to the upper glass coverslip of the chamber, and maximize the air exchanges for the cells. The chamber is placed in the incubator for one hour, again, for the cells to grow back their flagella.

### Experimental protocol

After the last incubation phase, the chamber is placed in an inverted microscope from Olympus. The microscope is completed by two optical filters (red, wavelength 670 nm, and blue, wavelength 470 nm) to monitor the light conditions in which the cells evolve. First, two photophobic choc (darkness for 2 minutes followed by a red illumination at maximal intensity for 2 minutes followed by darkness for two minutes) are imposed to the cells. Second, the cells are let under red light at the desired intensity ($10^{19}$ photons/m$^2$/s) and then under blue light at the same intensity for 10 minutes, and again under red light for 10 minutes. Finally, the illumination is switched to blue light at the desired intensity, which marks the beginning of the comparative experiments. After switching to blue light and a lag time on the order of one minute, the cells adhere to the bottom glass coverslip and exhibit gliding motion. Their motion is recorded *via* bright-field microscopy.

---

* Contact author: nicolasfares@hotmail.fr
† Also at CBMN, UMR 5248, CNRS, Bordeaux INP, University of Bordeaux, Pessac, France
‡ Also at TreeFrog Therapeutics, 33600, Pessac, France.
§ Contact author: thomas.salez@cnrs.fr
¶ Contact author: antoine.allard@u-bordeaux.fr

### Super-diffusive-like behavior

The trajectories of the cells in the comparative experiments are analyzed, leading to observables like in-plane mean squared displacements (MSDs) $\langle \delta_\tau r^2 \rangle$ and probability distribution functions (PDFs) $P(\delta_\tau r)$ of in-plane displacements $\delta_\tau r$ over a time $\tau$. The latter two observables are displayed in Fig. S1. As opposed to the main document (see Fig. 3 therein), averages (denoted by $\langle \cdot \rangle$) are performed on both time and the population of cells. The behavior discussed in the main document are retrieved in those comparative experiments. Indeed, MSDs grow as $\tau^\beta$ with $\beta \simeq 1.25$ (see Fig. S1A). Moreover, the PDFs of displacements follow Lorentzian-like distributions (see Fig. S1B), as in the main document. Besides, this result is time-invariant since the shape of the PDFs does not depend on the time lag $\tau$ considered (see Fig. S2).

## II. MIE HOLOGRAPHY AND GLIDING MOTILITY

### Spherical-homogeneous-alga approximation

As explained in the main text, tracking single cells *via* Mie holography relies on the approximate consideration of cells as homogeneous and spherical. Measured radii $a$ and refractive indices $n_{\mathrm{p}}$ are displayed in Fig. S3A. The radii are in fair agreement with previous measurements from the comparative experiments on groups of cells, which are also displayed in Fig. S3A, and both sets of experiments fall in the expected radius ballpark [38,53] (main document). Furthermore, the measured refractive indices, with values around 1.4 as shown in Fig. S3B, are also in the expected ballpark [52,53] (main document).

### Measurements in the normal direction

Because of the uncertainty on the measured $z$-positions (discussed in the main document around Fig. 1 in the main document), observables measured in the $z$-direction, while cells glide and stochastically oscillate between two positions, were not discussed in the main document. Nevertheless, they are shown here for the sake of completeness.

Firstly, the PDFs $P(\delta_\tau z)$ of normal displacements $\delta_\tau z$ over a time $\tau$ are shown in Fig. S4A. As evidenced by the linear slopes in a log-linear scale, the displacements are exponentially distributed. Secondly, the protocol to infer forces explained in the main document in the $r$-direction (see Eq. 2 of the main document, replacing $r$ by $z$) is repeated in the $z$-direction. Results are displayed in Fig. S4B-D. A $r$-trajectory is recalled in panel B, and the $z$-MSDs are displayed in panel C, either when the cells stay at one location or move from one position to the other. The resulting forces, highlighted in panel D, are on the order of the piconewton.

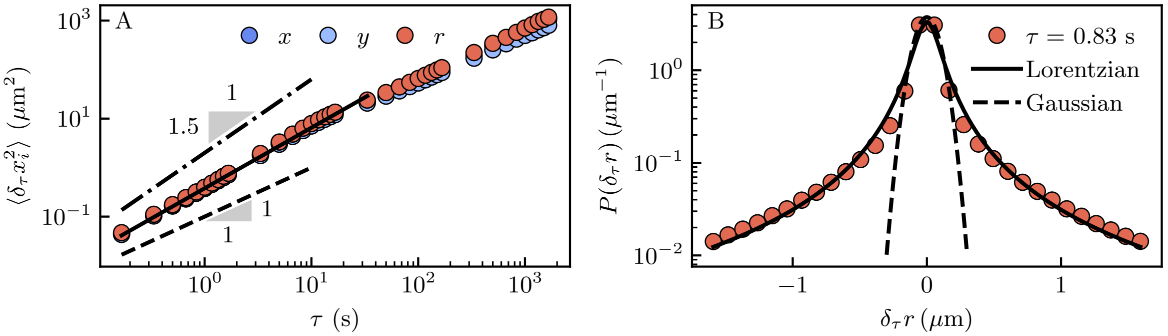


Figure S1: Gliding cells exhibit a super-diffusive-like behavior. In the panels, the disks correspond to experimental data, inferred from the comparative experiments described in Section I of the Supplementary Information. (A) In-plane mean squared displacements (MSDs) $\langle \delta_\tau x_i^2 \rangle$ as a function of the time increment $\tau$, in the directions $x_i = x$ (blue disks), $x_i = y$ (lighter-blue disks), and $x_i = r$ (red disks), with $r = \sqrt{(x - x(0))^2 + (y - y(0))^2}$. The black lines are guides to the eye. (B) Probability distribution function (PDF) $P(\delta_\tau r)$ of observing in-plane displacements $\delta_\tau r$ over a lag time $\tau = 0.83\,\text{s}$. The solid and dashed lines are, respectively, Lorentzian and Gaussian guides to the eye.

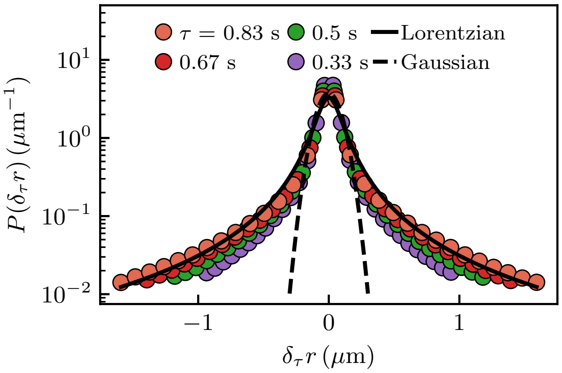


Figure S2: Time-dependency of the shape of the PDFs $P(\delta_\tau r)$ of in-plane displacements $\delta_\tau r$. PDFs are computed for several lag times $\tau$, which are indicated in legend. The red disks and related black lines correspond to Fig. S1B.

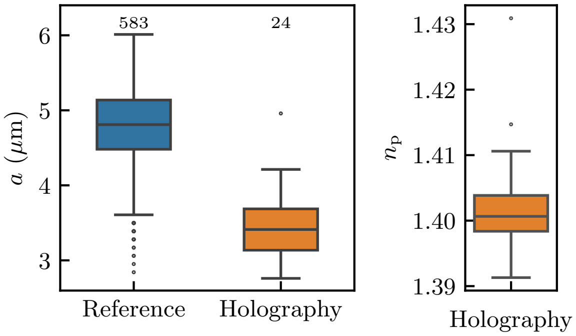


Figure S3: Effective physical properties of *C. reinhardtii.* (A) Effective radius $a$ of the cells, as measured by holography (orange) and from the comparative experiments (blue). (B) Effective refractive index $n_{\mathrm{p}}$ of the cells, as measured by holography.

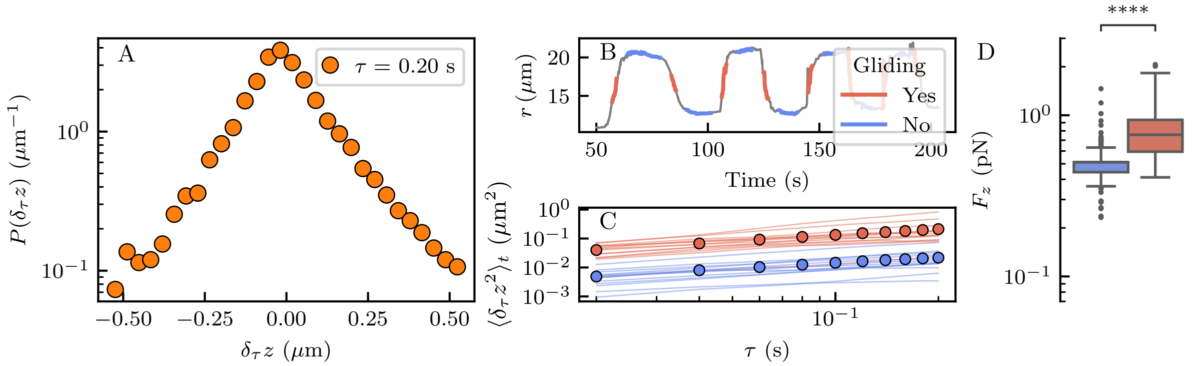


Figure S4: Dynamics of the cells in the direction normal to the glass wall on which they adhere. (A) Probability distribution function (PDF) $P(\delta_\tau z)$ of observing in-plane displacements $\delta_\tau z$ over a lag time $\tau = 0.2\,$s. (B) In-plane $r$-coordinate as a function of time of one cell. The colors highlights periods when the cell stays at one location (blue) or when the cell moves from one position to the other (red). (C) MSDs $\langle \delta_\tau z^2 \rangle$ in the $z$-direction, for both periods highlighted in panel B. (D) Normal force $F_z$ acting on the cell's body, for both periods highlighted in panel B. Forces are inferred from Eq. 2 of the main document (replacing $r$ by $z$).
